# Supplementary material for: CaSPR: Learning Canonical Spatiotemporal Point Cloud Representations
Source: arXiv:2008.02792 source file (2020-11-11)
Supplement: Supplementary file 1 [file disentangle.tex]

\stepcounter{appendixfigure}
\begin{wrapfigure}{r}{0.45\textwidth}
    \vspace{-13mm}
\includegraphics[width=0.45\textwidth]{appendix/images/supp_disentangle.png}\vspace{-4mm}
    \caption{Disentanglement examples on deforming cars data.}\vspace{-3mm}
    \label{appendix:fig:disentangle}
    \vspace{-6mm}
\end{wrapfigure}
